# Supplementary material for: HorizonNet: Learning Room Layout with 1D Representation and Pano Stretch Data Augmentation
Source: arXiv:1901.03861 source file (2019-04-06)
Supplement: Supplementary file 1 [file supp.tex]

\documentclass[10pt,onecolumn,letterpaper]{article}

\usepackage{cvpr}
\usepackage{times}
\usepackage{epsfig}
\usepackage{graphicx}
\usepackage{amsmath}
\usepackage{amssymb}
\usepackage{xcolor}
\usepackage{ifthen}
\usepackage{caption}
\usepackage{makecell}
\usepackage{textcomp}
\usepackage{array}
\usepackage{mathtools}
\usepackage{subcaption}
\usepackage{multirow}

\DeclareMathAlphabet\mathbfcal{OMS}{cmsy}{b}{n}

\makeatletter
\renewcommand{\paragraph}{%
  \@startsection{paragraph}{4}%
  {\z@}{0.5em \@plus 0ex \@minus 0ex}{0em}%
  {\normalfont\normalsize\bfseries}%
}
\makeatother

\captionsetup[table]{labelformat=simple, labelsep=period}

% Each member scope visulize in different color
\definecolor{red}{rgb}{0.9,0.1,0}
\definecolor{slateblue}{rgb}{0.7,0.35,0.9}
\definecolor{green}{rgb}{0, 0.4, 0}
\definecolor{orange}{rgb}{0.5, 0.25, 0}
\definecolor{mahogany}{rgb}{0.75, 0.25, 0.0}
\definecolor{purple}{rgb}{0.3, 0, 0.3}
% \definecolor{purple}{rgb}{0, 0, 0}
\definecolor{darkgreen}{rgb}{0, 0.4, 0}
\definecolor{frenchblue}{rgb}{0.0, 0.45, 0.73}
\definecolor{blue}{rgb}{0.0, 0.0, 1.0}
\definecolor{goldenrod}{rgb}{0.85, 0.65, 0.13}
\newboolean{revising}
\setboolean{revising}{false}
\ifthenelse{\boolean{revising}}
{
    \newcommand{\ignore}[1]{}

} {
    \newcommand{\ignore}[1]{}

}

% Include other packages here, before hyperref.

% If you comment hyperref and then uncomment it, you should delete
% egpaper.aux before re-running latex.  (Or just hit 'q' on the first latex
% run, let it finish, and you should be clear).
\usepackage[pagebackref=true,breaklinks=true,letterpaper=true,colorlinks,bookmarks=false]{hyperref}

\cvprfinalcopy % *** Uncomment this line for the final submission

 % *** Enter the CVPR Paper ID here

% Pages are numbered in submission mode, and unnumbered in camera-ready
\ifcvprfinal\pagestyle{empty}\fi
\begin{document}

%%%%%%%%% TITLE
% \newcommand{\modelname}{\text{HorizonNet}\xspace}
\title{Supplemental Materials of HorizonNet\vspace{-2.0cm}}

\maketitle
\thispagestyle{empty}

%%%%%%%%% BODY TEXT
\input{main/supp_sem.tex}

\input{main/supp_cuboid.tex}

\newpage

\input{main/supp_noncuboid.tex}

\clearpage

{\small
\bibliographystyle{ieee}
\bibliography{layout}
}

\end{document}
